# Supplementary material for: Properties of coplanar periodic electrodes in confined spaces: Case of two-dimensional diffusion
Source: arXiv:1802.00120 source file (2018-02-12)
Supplement: Supplementary file 1 [file text-additional_proofs.tex]

% !TeX root = article
% !TeX encoding = utf8
% !TeX spellcheck = en_US

\section{Additional proofs}

\subsection{Lemma \ref{coplanar:lem:g-h}}

In the proof below it is found how to obtain the principal parts
$\tilde{G}(z,s)$ and $\tilde{G}(z,s)^{-1}$ of $G(z,s)$ and $G(z,s)^{-1}$ through residues.

Since the number of poles of $G(z,s)$ and $G(z,s)^{-1}$ is infinite,
the the principal parts $\tilde{G}(z,s)$ and $\tilde{G}(z,s)^{-1}$
may not agree with the original functions $G(z,s)$ and $G(z,s)^{-1}$.

The agreement between $F(z,s) - \tilde{F}(z,s)$ with $F \in \{G, G^{-1}\}$ has to be verified
by applying \wikipedia{Mittag-Leffler's theorem}.
First take the difference $D(z,s) = F(z,s) - \tilde{F}(z,s)$, which is an entire function,
since the singularities are removed by substracting the principal part.
Next, we make use of \wikipedia{Liouville's theorem (complex analysis)},
by checking that $D(z,s)$ is bounded.
If it is bounded, then it means that $D(z,s)$ does not depend on $s$, that is $D(z,s) = f(z)$,
which means that $F(z,s) = f(z) + \tilde{F}(z,s)$.
If we are even more lucky, we may be able to find that $f(z) = 0$.

Below: How to find the principal parts of $\tilde{G}(z,s)$ and $\tilde{G}(z,s)^{-1}$.

\begin{proof}
	First recall the product expansions of $\sinh()$ and $\cosh()$
	\cite[{Eqs. (\dlmf[E]{4.36.}{1})} and {(\dlmf[E]{4.36.}{2})}]{dlmf}
	\begin{subequations}
		\begin{align}
		\sinh(\bm{u}) &=
		\bm{u} \prod_{k=1}^{+\infty} \left( 1 + \frac{\bm{u}^{2}}{k^{2} \pi^{2}} \right)
		\\
		\cosh(\bm{u}) &=
		\prod_{\ell=1}^{+\infty} \left(
		1 + \frac{4 \bm{u}^{2}}{(2\ell - 1)^{2} \pi^{2}}
		\right)
		\end{align}
	\end{subequations}
	and replace them in the expression for $G(z,s)$ and $G(z,s)^{-1}$ Eq. (\ref{coplanar:eqn:G}).	
	\begin{subequations}
		\begin{align}
			G(z,s) &=
			\frac{
				\cosh(\sqrt{s}\,z)/H
			}{
				\displaystyle
				s \prod_{k=1}^{+\infty} \left( 1 + \frac{s H^{2}}{k^{2} \pi^{2}} \right)
			}
			\\
			G(z,s)^{-1} &=
			\frac{
				\sqrt{s} \sinh(\sqrt{s}\, H)
			}{
				\displaystyle
				\prod_{\ell=1}^{+\infty} \left(
				1 + \frac{4s\, z^{2}}{(2\ell - 1)^{2} \pi^{2}}
				\right)
			}
		\end{align}
	\end{subequations}
	Here one can notice that both expressions have only real poles of multiplicity one
	\begin{subequations}
		\begin{align}
			s_{k} &= -k^{2} \frac{\pi^{2}}{H^{2}},& k &= 0, 1, 2, \ldots
			\\
			s_{\ell} &= -(2\ell - 1)^{2} \frac{\pi^{2}}{4z^{2}},& \ell &= 1, 2, \ldots
		\end{align}
	\end{subequations}
	where $s_{k}$ correspond to the poles of $G(z,s)$ and
	$s_{\ell}$ correspond to the poles of $G(z,s)^{-1}$
	(which are also the zeros of $G(z,s)$).
	This leads to the following partial fractions expansion
	\begin{subequations}
		\begin{align}
			\tilde{G}(z,s) &= \sum_{k=0}^{+\infty} \frac{A_{k}}{s - s_{k}}, &
			A_{k} &= \lim_{s \to s_{k}} (s - s_{k}) G(z,s)
			\\
			\tilde{G}(z,s)^{-1} &= \sum_{\ell=1}^{+\infty} \frac{B_{\ell}}{s - s_{\ell}}, &
			B_{\ell} &= \lim_{s \to s_{\ell}} (s - s_{\ell}) G(z,s)^{-1}
		\end{align}
	\end{subequations}
	Taking their inverse Laplace transform leads to
	\begin{subequations}
		\begin{align}
			g(z,t) = \laplace^{-1} \tilde{G}(z,s)
			&= \sum_{k=0}^{+\infty} A_{k} \e^{s_{k} t}
			\\
			h(z,t) = \laplace^{-1} \tilde{G}(z,s)^{-1}
			&= \sum_{\ell=1}^{+\infty} B_{\ell} \e^{s_{\ell} t}
		\end{align}
	\end{subequations}
	This completes the main proof.
	The rest of the proof consists of computing the coefficients $A_{k}$ and $B_{\ell}$.

	The coefficient $A_{0}$ can be calculated directly taking the limit
	\begin{subequations}
		\begin{align}
			A_{0} &= \lim_{s \to 0} s
			\frac{
				\cosh(\sqrt{s}\, z)
			}{
				\sqrt{s} \sinh(\sqrt{s}\, H)
			}
			= \lim_{s \to 0} \frac{1}{H}
			\frac{
				\cosh(\sqrt{s}\, z)
			}{
				\sinh(\sqrt{s}\, H)/(\sqrt{s}\, H)
			}
			\\
			A_{0} &= \frac{1}{H}
		\end{align}
	\end{subequations}
	and the remaining coefficients $A_{k}$ and $B_{\ell}$ can be computed by using L'Hôpital rule as follows
	\begin{subequations}
		\begin{align}
			A_{k} &= \lim_{s \to s_{k}} (s - s_{k})
			\frac{
				\cosh(\sqrt{s}\, z)
			}{
				\sqrt{s} \sinh(\sqrt{s}\, H)
			}
			\\
			&= \lim_{s \to s_{k}}
			\frac{
				\cosh(\sqrt{s}\, z) + (s - s_{k}) \deriv{}{s} \cosh(\sqrt{s}\, z)
			}{
				\num{0,5} H \sinh(\sqrt{s}\, H) / (\sqrt{s}\, H)
				+ \num{0,5} H \cosh(\sqrt{s}\, H)
			}
			\\
			&= \frac{2}{H}
			\frac{
				\cosh(\sqrt{s_{k}}\, z)
			}{
				\cosh(\sqrt{s_{k}}\, H)
			}
			= \frac{2}{H}
			\frac{
				\cos(\sqrt{|s_{k}|}\, z)
			}{
				\cos(\sqrt{|s_{k}|}\, H)
			}
			= \frac{2}{H}
			\frac{
				\cos(\sqrt{|s_{k}|}\, z)
			}{
				(-1)^{k}
			}
			\\
			&= \frac{2}{H} (-1)^{k} \cos(\sqrt{|s_{k}|}\, z)
		\end{align}
	\end{subequations}

	\begin{subequations}
		\begin{align}
			B_{\ell} &= \lim_{s \to s_{\ell}} (s - s_{\ell})
			\frac{
				\sqrt{s} \sinh(\sqrt{s}\, H)
			}{
				\cosh(\sqrt{s}\, z)
			}
			\\
			&= \lim_{s \to s_{\ell}}
			\frac{
				\sqrt{s} \sinh(\sqrt{s}\, H)
				+ (s - s_{\ell}) \deriv{}{s} \sqrt{s} \sinh(\sqrt{s}\, H)
			}{
				\num{0,5}z \sinh(\sqrt{s}\, z) / \sqrt{s}
			}
			\\
			&= \lim_{s \to s_{\ell}}
			\frac{
				2s \sinh(\sqrt{s}\, H)
			}{
				z \sinh(\sqrt{s}\, z)
			}
			= \frac{2}{z} s_{\ell} \frac{
				\sinh(\sqrt{s_{\ell}}\, H)
			}{
				\sinh(\sqrt{s_{\ell}}\, z)
			}
			\\
			&= \frac{2}{z} s_{\ell} \frac{
				\sin(\sqrt{|s_{\ell}|}\, H)
			}{
				\sin(\sqrt{|s_{\ell}|}\, z)
			}
			= \frac{2}{z} s_{\ell} \frac{
				\sin(\sqrt{|s_{\ell}|}\, H)
			}{
				(-1)^{\ell-1}
			}
			\\
			&= \frac{2}{z} |s_{\ell}| (-1)^{\ell} \sin(\sqrt{|s_{\ell}|}\, H)
		\end{align}
	\end{subequations}
\end{proof}
